# Supplementary material for: Few-shot Neural Radiance Fields Under Unconstrained Illumination
Source: arXiv:2303.11728 source file (2023-12-18)
Supplement: Supplementary file 1 [file extreme_6v.tex]

\begin{tabular}{l|ccc|ccc|ccc}
\toprule
 & \multicolumn{3}{c|}{Cafe} & \multicolumn{3}{c|}{Kitchen} & \multicolumn{3}{c}{Flower}\\ \midrule
  & SSIM $\uparrow$ & LPIPS $\downarrow$ & Abs Rel $\downarrow$ & SSIM $\uparrow$& LPIPS $\downarrow$ & Abs Rel $\downarrow$ & SSIM $\uparrow$& LPIPS $\downarrow$ & Abs Rel $\downarrow$\\ \midrule
NeRF-W~\cite{nerfinthewild} \ & - & - & -  & - & - & - & - & - & - \\
Ha-NeRF~\cite{HaNeRF} \ & - & - & -  & - & - & - & - & - & - \\
\midrule
RegNeRF~\cite{niemeyer2022regnerf}\ & 0.45 & 0.41 & 0.91  & 0.55 & 0.40 & 0.85 & 0.53 & 0.49 & 0.91 \\
FreeNeRF~\cite{yang2023freenerf} \ & 0.45 & 0.42 & 0.91  & 0.54 & 0.40 & 0.81 & 0.51 & 0.47 & 0.86 \\
\midrule
NeROIC-Geom.~\cite{kuang2022neroic}\ & - & - & -  & - & - & - & - & - & - \\
%\midrule
\textbf{ExtremeNeRF (Ours)}\ & 0.49 & 0.37 & 0.91 & 0.61 & 0.35 & 0.79 & 0.58 & 0.42 & 0.84 \\
\bottomrule
\end{tabular}
